# Supplementary material for: Reality and Computation in Schubert Calculus
Source: arXiv:1307.1833 source file (2013-07-07)
Supplement: Supplementary file 1 [file Appendices.tex]

\appendix
  %--------------------------------------------------------------------------------
  % Appendix A
  %--------------------------------------------------------------------------------
  \chapter{FIRST APPENDIX}
    \label{Appendix: First Appendix}
    %\input{./Chapters/AppendicesSections/FirstAppendix}

  %--------------------------------------------------------------------------------
  % Appendix B
  %--------------------------------------------------------------------------------
  \chapter{SECOND APPENDIX}
    \label{Appendix: Second Appendix}
