# Supplementary material for: Reality and Computation in Schubert Calculus
Source: arXiv:1307.1833 source file (2013-07-07)
Supplement: Supplementary file 2 [file FirstAppendix.tex]

Put your first appendix here.
